# Supplementary material for: FODVid: Flow-guided Object Discovery in Videos
Source: arXiv:2307.04392 source file (2023-07-10)
Supplement: Supplementary file 1 [file appendix.tex]

Extra sections go here.
